# Supplementary material for: COVID-19 Screening Using Residual Attention Network an Artificial Intelligence Approach
Source: arXiv:2006.16106 source file (2020-10-20)
Supplement: Supplementary file 1 [file appendix.tex]

\section{Appendix}
\label{sec:appendix}
